# Supplementary material for: What Leads to Administrative Bloat? A Dynamic Model of Administrative Cost and Waste
Source: arXiv:2412.15378 ancillary file (2026-06-01)
Supplement: Supplementary file 1 [file SI.pdf]

# Supplementary Information

## Contents

|          |                                                                                                            |          |
|----------|------------------------------------------------------------------------------------------------------------|----------|
| <b>1</b> | <b>Data and code availability</b>                                                                          | <b>1</b> |
| <b>2</b> | <b>Methods</b>                                                                                             | <b>1</b> |
| 2.1      | Determining equilibria and stability . . . . .                                                             | 1        |
| 2.2      | Simulation of the baseline behavioral model and parameters . . . . .                                       | 2        |
| 2.3      | Simulation for optimizing organization with discounting . . . . .                                          | 2        |
| <b>3</b> | <b>Results in the case of <math>k_c &gt; k_p</math> and critical transition at <math>k_c = k_p</math>.</b> | <b>2</b> |
| <b>4</b> | <b>Testing model robustness under partial process administration</b>                                       | <b>3</b> |
| <b>5</b> | <b>Multiple equilibria and path dependency</b>                                                             | <b>4</b> |

## 1 Data and code availability

Data on MIT administrative staff, students, and faculty are collected from the following two sources. Years 1985–2007 are collected from MIT Faculty News Letter Vol. XX No. 1, September/October 2007. Years 2013–2023 are from MIT Institutional Research website: <https://ir.mit.edu/data-browser>.

The data analyzed, and simulation code used in this study are included in the manuscript submission as a supplementary file.

## 2 Methods

### 2.1 Determining equilibria and stability

After including the derived flow rates of the main text in Equation 1, our model is characterized by the following system of differential equations:

$$\frac{dR_u}{dt} = \frac{(w - w_A)c}{k_c} - \frac{R_u}{T_d} \quad (\text{S1})$$

$$\frac{dR_o}{dt} = \frac{R_u}{T_d} - \frac{(w - w_A)p}{k_p} \frac{R_o}{R_u + R_o} \quad (\text{S2})$$

where  $w_A = k_A(R_u + R_o)$ , and  $c$  and  $p$  are later derived to be functions of  $R_u$  and  $R_o$ . We solve for equilibria of the system by solving for  $R_u$  and  $R_o$  where  $\frac{dR_u}{dt} = \frac{dR_o}{dt} = 0$ . We do so computationally in Python 3 language. We evaluate the stability of each equilibrium using the eigenvalue of the Jacobian matrix at the equilibrium. Negative eigenvalues correspond to stable equilibria; positive eigenvalues correspond to unstable equilibria.

## 2.2 Simulation of the baseline behavioral model and parameters

We simulate the system of differential equations using Euler’s method, written in Python 3 language. The default parameters in Table 1 of the main text are obtained by considering an organization of 50 employees where processes become obsolete in 60 months (6 years) on average. We assume that it would take a team of three people one full workday to create a new process (24 hours), whereas it would take three times the workload to remove a previously implemented process (72 hours). We also assume the organization as a whole spends 15 hours per month to administer each process (parameter  $k_A$ ), which is about 18 minutes per employee per process per month. As desired production, creation propensity, and pruning propensity are between 0 and 1, we choose 0.5 as the default value for those parameters. We choose a value of 0.05 for the process efficacy—taking approximately 14 processes to reduce the problem space of the firm by half. We assume the returns of direct production and useful processes are diminishing and favor direct production.

In the simulation of Figure 3 in the main text, Panel (A) uses the default values, and panel (B) has the changes  $\gamma_c = 0.9$  and  $\gamma_p = 0.1$ . The company performance was calculated with a return on direct production of  $\alpha = 0.8$  and a return on useful processes of  $\beta = 0.5$ .

Regarding Figure 4 of the main text, panel (A) uses the default parameters in Table 1. Panel (B) uses three different  $T_d$  values, as noted in the figure.

The environmental shock simulation of Figure 5 of the main text simulates a shock lasting for 12 months, where the time for process obsolescence is shortened to 1.2 months in panel A and 0.75 months in panel B. The parameters used are  $\gamma_c = 0.75$  and  $\gamma_p = 0.3$  in both panels. The rest of the parameters are the same as those in Table 1.

In the main text, the equilibrium analysis in Figure 6 (A) uses the same parameter values as Table 1. Panel (B) changes the  $k_p$  value to be six times that of panel (A).

## 2.3 Simulation for optimizing organization with discounting

To consider the optimal management strategies, we determine the maximal utility of the firm ( $\mathcal{U}$ ) exponentially discounted over time. The discounted utility at time  $t$  is  $\mathcal{U}_t^O = \mathcal{U}e^{-rt}$ , where  $r$  is the discount rate. Given some time-horizon  $T$  and an update time  $\tau \leq T$ , we calculate the optimal strategy of the firm by determining the resource allocation which maximizes the firm’s discounted utility over  $T$  months. This allocation strategy is then employed for  $\tau$  months after which the optimal allocation is reevaluated and implemented for the next  $\tau$  months. We continue in this manner until the firm has been simulated for the entire period  $T$ . For the results shown in Figure 7 of the main text, we assume that the firm updates their strategy via quarterly meetings once every three months. Therefore, we use  $\tau = 3$ . We assume that the organization based their decisions on the discounted utility over the next ten years. Therefore,  $T = 120$ . For the model parameters, we use their default values (as seen in Table 1 of the main text) in all three panels of Figure 7. In panel (A), we take  $r = 0$ . In panel (B),  $r = 0.21$ . In panel (C), we use  $T = 120$  and  $\tau = 3$  and run the simulation until the resource allocations approach a stable equilibrium.

The utility of the firm (prior to discounting) at a given time is given by a Cobb-Douglas production function of the work allocated towards direct production,  $w_D$ , and the number of useful processes,  $R_u$ . This resulting utility is  $\mathcal{U}(t) = (w_D(t))^\alpha (R_u(t))^\beta$ , where we make the time dependence explicit. In all of our results, we take  $\alpha = 0.8$  and  $\beta = 0.5$ . Therefore, at each reassessment period  $h = n\tau$  where  $n$  is some whole number, the optimizer adopts the strategy  $(\tilde{d}, \gamma_c, \gamma_p)$  which maximizes the integral  $\int_h^{h+\tau} (w_D(t))^\alpha (R_u(t))^\beta e^{-rt} dt$ . In our optimization results, we use  $T_d = 10$ .

## 3 Results in the case of $k_c > k_p$ and critical transition at $k_c = k_p$ .

The main text of our manuscript focuses on scenarios in which process pruning is more expensive than creation, as is typical in real-world organizations. Our model also predicts that if the cost of process creation

( $k_c$ ) is greater than that of pruning ( $k_p$ ), then the only stable equilibrium that occurs is a sustainable equilibrium. Below, we outline an analysis that shows why a critical transition occurs at  $k_c = k_p$ .

We analyze this critical transition by considering the Jacobian matrix of the system of differential equation, whose eigenvalues indicate the stability of equilibria. If both eigenvalues are negative, the equilibrium is stable, and if there is at least one positive eigenvalue, it is unstable.

We may first conclude that the run-away bloat outcome ( $R_u = 0, R_o = w/k_A$ ) is an equilibrium solution by substituting these values of  $R_u$  and  $R_o$  into the system of differential equations and observing that the derivatives of the stock variables,  $dR_u/dt$  and  $dR_o/dt$ , are indeed equal to zero. We then evaluate the Jacobian matrix at this position and determine the two eigenvalues are

$$\lambda_1 = -\frac{1}{T_d}, \quad \lambda_2 = \frac{k_A}{2 + \bar{d}} \left( \frac{1}{k_p} - \frac{1}{k_c} \right) \quad (\text{S3})$$

Because  $T_d$  is positive, the first eigenvalue  $\lambda_1$  is always negative. Therefore, the administrative bloat position only changes stability when  $\lambda_2$  switches signs. Since  $k_A$  and  $\bar{d}$  are both positive, we see that  $\lambda_2$  can only change signs at  $k_p = k_c$ . If  $k_p < k_c$ , then  $\lambda_2$  is positive, and the administrative bloat position is unstable. If  $k_p > k_c$  (reflecting real-world organizations), then  $\lambda_2$  is negative, and the administrative bloat position is stable.

## 4 Testing model robustness under partial process administration

We consider the question: what happens if the firm does not administer all of its processes? More specifically, does the observed administrative bloat still occur? To answer this question, we include an additional multiplicative term in the model which denotes the proportion of processes administered. We assume the proportion of administered processes is a monotonically decreasing function of the number of processes. That is, we assume that as a firm has more processes to administer, employees will cut more corners. We assume the following mathematical form:

$$f(w_A) = e^{-b(w_A/w)} \quad (\text{S4})$$

where  $f$  is the fraction of processes administered, and  $w_A = k_A(R_u + R_o)$  is the administrative costs without partial administration. This additional term can be incorporated in the system of governing equations in the following manner:

$$\frac{dR_u}{dt} = \frac{(w - w_A f(w_A) c)}{k_c} - \frac{R_u}{T_d} \quad (\text{S5})$$

$$\frac{dR_o}{dt} = \frac{R_u}{T_d} - \frac{(w - w_A f(w_A)) p}{k_p} \frac{R_o}{R_u + R_o} \quad (\text{S6})$$

The formulations for allocation to process creating and pruning are adjusted accordingly to reflect the partial enforcement:  $\tilde{c} = \gamma_c^{af(w_A)R_u}$  and  $\tilde{p} = ((f(w_A)w_A/w)^{-\log(\gamma_p)})$ . Consistent with our model in the main text, it is assumed in this formulation that individuals do not have knowledge of whether a process is obsolete or useful.

The prediction of this model for the parameter region separating the stable equilibrium and run-away bloat is shown in Figure S1. The left panel is for parameter  $b = 0.1$ , and the right panel is for  $b = 1$ . A greater  $b$  value represents a greater portion of processes not administered. The critical threshold between the two types of behavior still occurs, although this threshold is adversely affected as the proportion of the administered process decreases.

Intuitively, one may expect that not administering a subset of the firm's processes would decrease the organization's administrative costs. However, by not administering processes, the organization's problem remains unresolved, and it feels the same push toward process creation that it did previously. So a partially

enforcing organization will have more processes (including both administered and ignored) than its fully administering counterpart. Indeed, we see this in our results in Figure S1.

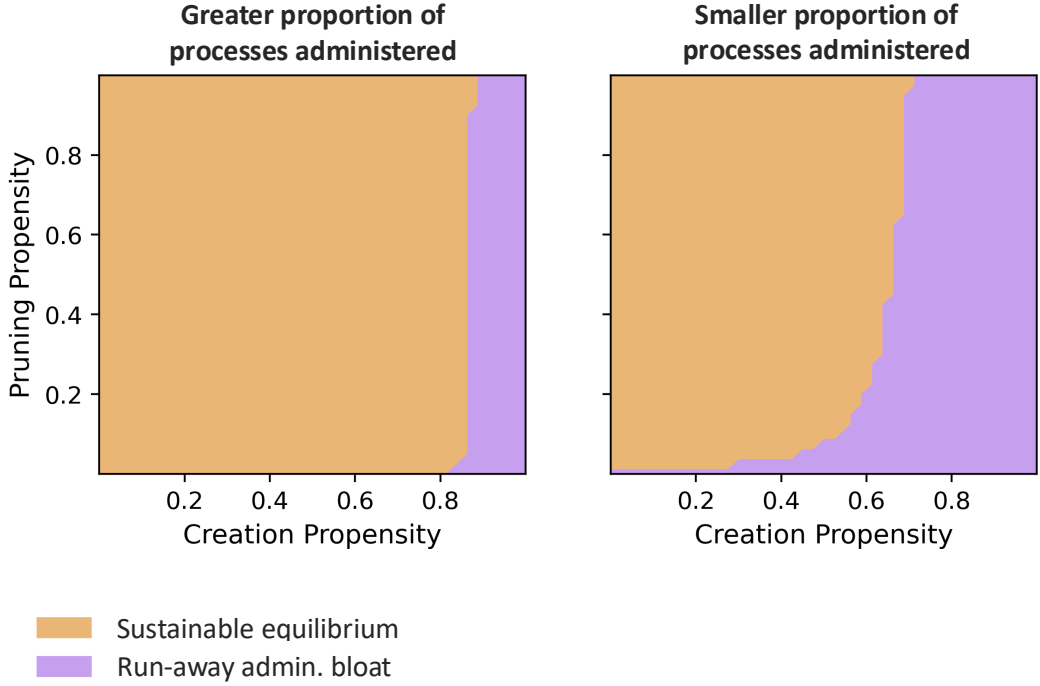

Figure S1: Model predictions for parameter regions separating the stable equilibrium and run-away bloat when considering a proportion of processes are not administered. The left panel is for parameter  $b = 0.1$  (more processes administered), and the right panel is for  $b = 1$  (fewer processes administered)

## 5 Multiple equilibria and path dependency

We note the dependence of the firm's outcome on its history. The possible dynamics of the system are illustrated as vector plots in Figure. S2. The two axes show the two important state variables, useful and obsolete processes ( $R_u$  and  $R_o$ , respectively). Since the number of total processes ( $R_u + R_o$ ) is limited by the resource of the organization, only the triangular region below the diagonal is possible. Arrows indicate the directions and magnitudes of change for the system starting at the state where the arrows originate. Where the arrows converge indicate stable equilibria. Panel (A) shows the scenario where only the sustainable equilibrium outcome is possible. Panel (B) shows when both sustainable equilibrium and run-away bloat are both possible. Which equilibrium is reached depends on the initial conditions of the system. Organizations growing from few initial processes evolve to the sustainable equilibrium. Panel (C) shows the scenario where only the run-away bloat is possible. Since most organizations tend to grow from small to large, we categorize both (A) and (B) as sustainable equilibrium outcome in the main text and (C) as the run-away bloat outcome.

The parameter values used in the panels of Figure 2 are (A)  $\gamma_c = 0.5$ ,  $\gamma_p = 0.15$ , and  $k_P = 20$ ; (B)  $\gamma_c = 0.8$ ,  $\gamma_p = 0.15$ ,  $k_P = 40$ ; and (C)  $\gamma_c = 0.9$ ,  $\gamma_p = 0.15$ , and  $k_P = 40$ . The value of  $T_d$  was decreased to 10 for all of these plots to emphasize the dynamics in the illustration (this does not change the position of the equilibria).

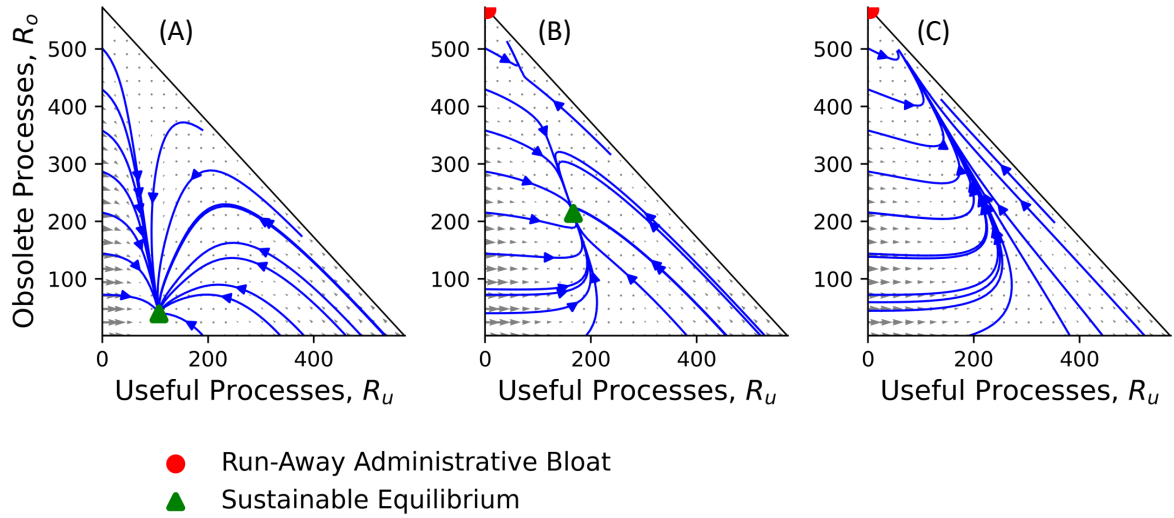

Figure S2: Vector fields illustrating the three types of system outcomes. Arrows indicate directions and magnitudes of change given the current state of the system. Blue lines show examples of system trajectories. (A) Only sustainable equilibrium possible. (B) Both sustainable equilibrium and runaway growth are possible, depending on starting conditions. (C) Only run-away growth is possible regardless of the starting point of the system.
